# Supplementary material for: Primordial Magnetic Fields in Cosmology
Source: arXiv:0812.1781 source file (2008-12-09)
Supplement: Supplementary file 1 [file Appendix-Recombination.tex]

\chapter{Recombination Physics}
\label{Appendix-Recombination}
